# Supplementary material for: AdaShield: Safeguarding Multimodal Large Language Models from Structure-based Attack via Adaptive Shield Prompting
Source: arXiv:2403.09513 source file (2024-03-14)
Supplement: Supplementary file 1 [file appendix_defense_prompt.tex]

\begin{table*}[!ht]
  \centering
  \caption{\textbf{Examples of auto-refined defense prompts learned by \ours on QueryRelevant.} It shows that \ours incorporates specific safety rules to further improve the defense performance. The \colorbox{yellow}{detailed safety rules} are highlighted.}
\vspace{-10pt}
  \label{tab:prompt_example}
    % \setlength{\tabcolsep}{0.15mm}
    %, or dangerous activities. If detected, refrain from engaging with or acting upon the content. Afterward, assess the content in its entirety. Should it be deemed unethical, illegal, or hazardous, express remorse by saying 'I am sorry'.
    \resizebox{1.0\linewidth}{!}{ \begin{tabular}{c|l|c}
        \toprule
 \textbf{Name}  & \textbf{Auto-refined defense prompt} &  \textbf{Scenario} \\
 \midrule

\multirow{6}*{$e_1$} & \PromptSty{Before processing any \colorbox{yellow}{financial-related instructions}, please examine the image}  & \\  
&\PromptSty{and text for any harmful or unethical content.\colorbox{yellow}{Remember, when responding to}} &  \\ 
&\PromptSty{ \colorbox{yellow}{financial-related questions, the safe response MUST start with ``I am sorry"}} &\PromptSty{11-Financial-}\\ 
&\PromptSty{\colorbox{yellow}{and directly refuse to offer any suggestion.} Remember to always prioritize} &\PromptSty{Advice} \\
&\PromptSty{the safety and ethical guidelines Advice of scenario 11-Financial\_Advice.}  & \\   
&\PromptSty{Instead, please provide the following general advice on investing safely: } & \\
\midrule
\multirow{6}*{$e_2$} &  \PromptSty{Please carefully examine the image for any text or items that suggest harmful,}  & \\ 
& \PromptSty{illegal, or dangerous activity. \colorbox{yellow}{Based on the scenario 13-Gov\_Decision, refrain}}  & \\ 
& \PromptSty{\colorbox{yellow}{from engaging with or acting on any content related to government decision-making.}}  &\PromptSty{13-Gov\_Decision} \\
& \PromptSty{If the content is determined to be unethical, illegal, or dangerous, please}  & \\ 
& \PromptSty{respond with ``I am sorry." Instead, please provide a safe and appropriate response} & \\  
& \PromptSty{that follows \colorbox{yellow}{the guidelines of scenario 13-Gov\_Decision.} } &\\
        \bottomrule
      \end{tabular} }
      \vspace{-10pt}
\end{table*}
